# Supplementary material for: Learning Semantically Coherent and Reusable Kernels in Convolution Neural Nets for Sentence Classification
Source: arXiv:1608.00466 source file (2016-10-10)
Supplement: Supplementary file 2 [file appendix_new.tex]

\newpage
\appendix
\section{Supplemental Material}

\textbf{Datasets Details}
\begin{itemize}
    \item \textbf{Movie Review} : Movie review dataset contains 5331 positive and 5331 negative reviews introduced in \cite{pang2005}\footnote{https://www.cs.cornell.edu/people/pabo/movie-review-data/}. The problem is a binary classification problem 
    \item \textbf{SUBJ} : The dataset contains 5000 subjective and 5000 objective sentences introduced in \cite{pang2004sentimental}\footnote{https://www.cs.cornell.edu/people/pabo/movie-review-data/}. The problem is to classify the given sentence as subjective or objective.
    \item \textbf{SST1} : Stanford Sentiment Treebank 1 is an extension to MR (Movie Review) with the Train/Test/Dev splits. The numbers are given in the table. The dataset is a fine grained version with 5 labels(very positive, positive, neutral, negative and very negative) introduced in \cite{socher2013recursive} \footnote{http://nlp.stanford.edu/sentiment/}
    \item \textbf{SST2} : Stanford Sentiment Treebank 2 is a subset to SST1 with neutral reviews removed, positive and very positive labelled as positive, negative and very negative labelled as negative. The problem solved is a binary classification problem.
    \item \textbf{IMDB} : Internet Movie DataBase is the large movie review dataset with 25000 train and 25000 test samples. The problem is binary classification problem introduced in \cite{maas-EtAl:2011:ACL-HLT2011}\footnote{http://ai.stanford.edu/~amaas/data/sentiment/}. The dataset also contains ratings from 1 to 10 given by the user.
\end{itemize}
